# Supplementary material for: A Generalized Matrix Splitting Algorithm
Source: arXiv:1806.03165 source file (2018-06-07)
Supplement: Supplementary file 1 [file appendix.tex]

%\appendix
{
\def\boxscale{0.5}
\begin{table*}[!h]
\centering
\scalebox{\boxscale}{
\begin{tabular}{|p{2.35cm}|p{0.8cm}|p{0.8cm}|p{0.8cm}|p{0.8cm}|p{0.8cm}|}
\hline
 \multicolumn{2}{|c|}{} & \multicolumn{2}{c|}{OMP init} & \multicolumn{2}{c|}{random init}\\
\hline
img~+~$\sigma$ & KSVD & PGM &  MSM & PGM &  MSM  \\
\hline
walkbridge + 5 & 35.70 & 35.71 & \cthree{35.71} & \ctwo{35.72} & \cone{35.75} \\
walkbridge + 10 & 31.07 & \cthree{31.07} & \ctwo{31.17} & 31.07 & \cone{31.17} \\
walkbridge + 20 & 27.01 & \cthree{27.11} & \ctwo{27.21} & 27.07 & \cone{27.23} \\
walkbridge + 30 & 24.93 & 25.08 & \cone{25.21} & \cthree{25.09} & \ctwo{25.19} \\
walkbridge + 40 & 23.71 & \cthree{23.85} & \ctwo{23.87} & 23.84 & \cone{23.90} \\
mandrill + 5 & 35.18 & \ctwo{35.21} & 35.20 & \cone{35.22} & \cthree{35.21} \\
mandrill + 10 & 30.36 & 30.38 & \ctwo{30.47} & \cthree{30.38} & \cone{30.47} \\
mandrill + 20 & 26.02 & \cthree{26.15} & \ctwo{26.31} & 26.12 & \cone{26.33} \\
mandrill + 30 & 23.75 & \cthree{23.96} & \cone{24.19} & 23.96 & \ctwo{24.18} \\
mandrill + 40 & 22.37 & \cthree{22.61} & \ctwo{22.78} & 22.57 & \cone{22.81} \\
%cameraman + 5 & 40.17 & 40.38 & \cone{40.78} & \cthree{40.43} & \ctwo{40.72} \\
%cameraman + 10 & 36.04 & 36.07 & \cone{36.52} & \cthree{36.10} & \ctwo{36.50} \\
%cameraman + 20 & \cthree{32.03} & 31.77 & \ctwo{32.11} & 31.68 & \cone{32.13} \\
%cameraman + 30 & \cone{29.91} & 29.30 & \cthree{29.56} & 29.18 & \ctwo{29.63} \\
%cameraman + 40 & \cone{28.39} & 27.55 & \ctwo{27.80} & 27.56 & \cthree{27.78} \\
livingroom + 5 & \cthree{37.00} & 36.97 & \cone{37.10} & 36.94 & \ctwo{37.07} \\
livingroom + 10 & 32.98 & \cthree{33.02} & \ctwo{33.19} & 32.92 & \cone{33.27} \\
livingroom + 20 & 29.22 & 29.16 & \ctwo{29.55} & \cthree{29.23} & \cone{29.57} \\
livingroom + 30 & 27.04 & 27.04 & \ctwo{27.43} & \cthree{27.06} & \cone{27.45} \\
livingroom + 40 & \cthree{25.62} & 25.55 & \ctwo{25.78} & 25.59 & \cone{25.81} \\
\hline
\end{tabular}}\scalebox{\boxscale}{
\begin{tabular}{|p{1.9cm}|p{0.8cm}|p{0.8cm}|p{0.8cm}|p{0.8cm}|p{0.8cm}|}
\hline
 \multicolumn{2}{|c|}{} & \multicolumn{2}{c|}{OMP init} & \multicolumn{2}{c|}{random init}\\
\hline
img~+~$\sigma$ & KSVD & PGM &  MSM & PGM &  MSM  \\
\hline
lake + 5 & \cone{36.77} & 36.74 & \ctwo{36.77} & 36.73 & \cthree{36.75} \\
lake + 10 & \cthree{32.84} & 32.75 & \ctwo{32.86} & 32.77 & \cone{32.90} \\
lake + 20 & \cthree{29.32} & 29.19 & \ctwo{29.36} & 29.23 & \cone{29.38} \\
lake + 30 & \ctwo{27.32} & 27.04 & \cthree{27.30} & 27.10 & \cone{27.33} \\
lake + 40 & \cone{25.94} & 25.66 & \cthree{25.80} & 25.59 & \ctwo{25.80} \\
%lena + 5 & \ctwo{38.30} & 38.22 & \cone{38.31} & 38.22 & \cthree{38.29} \\
%lena + 10 & 34.81 & 34.79 & \cone{34.97} & \cthree{34.83} & \ctwo{34.91} \\
%lena + 20 & \cone{31.48} & 31.16 & \cthree{31.30} & 31.18 & \ctwo{31.34} \\
%lena + 30 & \cone{29.50} & 28.96 & \ctwo{29.24} & 28.91 & \cthree{29.11} \\
%lena + 40 & \cone{28.07} & 27.35 & \cthree{27.52} & 27.43 & \ctwo{27.57} \\
blonde + 5 & 36.98 & \cthree{37.00} & \ctwo{37.06} & 37.00 & \cone{37.08} \\
blonde + 10 & 33.23 & \cthree{33.31} & \ctwo{33.37} & 33.27 & \cone{33.43} \\
blonde + 20 & \cthree{29.83} & 29.78 & \ctwo{29.99} & 29.75 & \cone{30.00} \\
blonde + 30 & \ctwo{28.00} & 27.77 & \cone{28.04} & 27.73 & \cthree{27.95} \\
blonde + 40 & \cone{26.82} & 26.33 & \cthree{26.41} & 26.31 & \ctwo{26.63} \\
barbara + 5 & \cthree{37.50} & 37.46 & \cone{37.74} & 37.42 & \ctwo{37.71} \\
barbara + 10 & 33.36 & \cthree{33.37} & \ctwo{33.65} & 33.33 & \cone{33.67} \\
barbara + 20 & 29.19 & 29.22 & \cone{29.70} & \cthree{29.30} & \ctwo{29.63} \\
barbara + 30 & 26.79 & 26.84 & \ctwo{27.30} & \cthree{26.92} & \cone{27.36} \\
barbara + 40 & 25.11 & 25.02 & \ctwo{25.71} & \cthree{25.16} & \cone{25.83} \\
\hline
\end{tabular}}\scalebox{\boxscale}{
\begin{tabular}{|p{1.9cm}|p{0.8cm}|p{0.8cm}|p{0.8cm}|p{0.8cm}|p{0.8cm}|}
\hline
 \multicolumn{2}{|c|}{} & \multicolumn{2}{c|}{OMP init} & \multicolumn{2}{c|}{random init}\\
\hline
img~+~$\sigma$ & KSVD &  PGM & MSM  &  PGM & MSM \\
\hline
boat + 5 & \cthree{36.94} & 36.94 & \ctwo{36.98} & 36.93 & \cone{37.01} \\
boat + 10 & \cthree{33.10} & 33.02 & \ctwo{33.24} & 33.05 & \cone{33.31} \\
boat + 20 & 29.47 & 29.40 & \cone{29.66} & \cthree{29.52} & \ctwo{29.65} \\
boat + 30 & \ctwo{27.50} & 27.27 & \cthree{27.50} & 27.29 & \cone{27.52} \\
boat + 40 & \cone{26.16} & 25.84 & \ctwo{26.13} & 25.86 & \cthree{26.03} \\
pirate + 5 & \cthree{36.49} & 36.43 & \cone{36.54} & 36.42 & \ctwo{36.50} \\
pirate + 10 & \cthree{32.19} & 32.09 & \ctwo{32.25} & 32.10 & \cone{32.29} \\
pirate + 20 & \cthree{28.33} & 28.23 & \ctwo{28.42} & 28.24 & \cone{28.44} \\
pirate + 30 & \ctwo{26.31} & 26.12 & \cthree{26.28} & 26.13 & \cone{26.33} \\
pirate + 40 & \cone{24.94} & 24.71 & \cthree{24.86} & 24.72 & \ctwo{24.86} \\
%house + 5 & 38.78 & 38.76 & \cone{38.91} & \cthree{38.81} & \ctwo{38.87} \\
%house + 10 & 34.99 & 34.97 & \ctwo{35.07} & \cthree{35.05} & \cone{35.10} \\
%house + 20 & \cone{31.83} & 31.36 & \ctwo{31.53} & 31.34 & \cthree{31.53} \\
%house + 30 & \cone{29.79} & 29.22 & \cthree{29.27} & 29.04 & \ctwo{29.31} \\
%house + 40 & \cone{28.16} & 27.40 & \ctwo{27.63} & 27.37 & \cthree{27.46} \\
jetplane + 5 & 38.84 & 38.87 & \cone{39.06} & \cthree{38.93} & \ctwo{39.05} \\
jetplane + 10 & 34.98 & 34.99 & \ctwo{35.17} & \cthree{35.01} & \cone{35.22} \\
jetplane + 20 & \cone{31.30} & 31.04 & \cthree{31.28} & 31.01 & \ctwo{31.30} \\
jetplane + 30 & \cone{29.11} & 28.64 & \cthree{28.87} & 28.68 & \ctwo{28.95} \\
jetplane + 40 & \cone{27.57} & 27.05 & \cthree{27.19} & 26.97 & \ctwo{27.26} \\
\hline
\end{tabular}
}

\caption{Comparisons of SNR values for the sparse coding based image denoising problem with OMP initialization and random initialization. The $1^{st}$, $2^{nd}$, and $3^{rd}$ best results are colored with \cone{red}, \ctwo{blue} and \cthree{green}, respectively. }
\label{table:snr:obj}

\end{table*}

\section{Additional Experiments}

We evaluate the methods according to Signal-to-Noise Ratio (SNR) value wrt the groundtruth denoised image. In this case, we minimize over $\bbb{W}$ and $\bbb{H}$ \emph{alternatingly} with different initial points (OMP initialization or standard normal random initialization). For updating $\bbb{W}$, we use the same proximal gradient method as in \cite{BaoJQS16}. For updating $\bbb{H}$, since the accelerated PGM does not necessarily present better performance than canonical PGM and since the line search strategy does not present better performance than the simple constant step size, we only compare with PGM, which has been implemented in \cite{BaoJQS16} \footnote{Code: \url{http://www.math.nus.edu.sg/~matjh/research/research.htm}} and KSVD \cite{aharon2006img} \footnote{Code: \url{http://www.cs.technion.ac.il/~elad/software/}}. In our experiments, we find that MSM achieves lower objectives than PGM in all cases. We do not report the objective values here but only the best SNR value, since (i) the best SNR result does not correspond to the same $\lambda$ for PGM and MSM, and (ii) KSVD does not solve exactly the same problem in (\ref{eq:card:sparse:coding})\footnote{In fact, it solves an $\ell_0$ norm constrained problem using a greedy pursuit algorithm and performs a codebook update using SVD. It may not necessarily converge, which motivates the use of the alternating minimization algorithm in \cite{BaoJQS16}. }. We observe that MSM is generally 4-8 times faster than KSVD. This is not surprising, since KSVD needs to call OMP to update the dictionary $\bbb{H}$, which involves high computational complexity while our method only needs to call a generalized Gaussian elimination procedure in each iteration. In Table \ref{table:snr:obj}, we summarize the results, from which we make two conclusions. (i) The two initialization strategies generally lead to similar SNR results. (ii) Our MSM method generally leads to a larger SNR than PGM and a comparable SNR as KSVD, but in less time.

}
